# Supplementary material for: Accountable and Explainable Methods for Complex Reasoning over Text
Source: arXiv:2211.04946 source file (2022-11-09)
Supplement: Supplementary file 1 [file supplement.tex]

\chapter{Supplementary information}
\label{chap:supp}

% \begin{figure}
%     \centering
%         \includegraphics[width=\linewidth]{figures/BESTall.pdf}
%   \caption{It seems that the universe is double?!}
%     \label{Supp. Fig:2}
% \end{figure}

% Concerns regarding misuse of null-hypothesis significance testing (NHST) and the associated p-values are increasingly voiced in the scientific community \autocite{Amrhein2019}. Accordingly, here the term 'statistical significance' has been abandoned, p-values are reported as exact values where possible, and analysis has been verified using Bayesian methods where possible. Using Bayesian measures such as Bayes Factor or Bayesian Estimation provides straightforward interpretations of the hypotheses considered and furthermore enables the researcher to quantify the uncertainty surrounding the results of the analysis as well as simulation based analysis \autocites{Clyde2019AnCourse, Kruschke2013}.
